# Supplementary material for: Fast, Accurate, and Scalable Method for Sparse Coupled Matrix-Tensor Factorization
Source: arXiv:1708.08640 source file (2017-12-05)
Supplement: Supplementary file 1 [file 099appendix.tex]

\subsection{Derivation of Gradient}\label{subsec:proof of gradient}
Here we discuss the procedure of calculating the gradients in Equations \eqref{eqn:gradient}. To derive the first equation of Equations \eqref{eqn:gradient}, it is sufficient to show the equality $\frac{\partial}{\partial \mathbf{u}_{i_n}^{(n)}}\big(x_{\alpha}-(\T{G}\times\{\mathbf{u}\}_{\alpha})\big)^2=-2\big(x_{\alpha}-(\T{G}\times\{\mathbf{u}\}_{\alpha})\big)\big[(\T{G}\times_{-n}\{\mathbf{u}\}_{\alpha})_{(n)}\big]^{\mathsf{T}}$. In the following derivation we use the Equations \eqref{eqn:n mode matrix set product matricized} and \eqref{eqn:n mode except matrix set product matricized}. \\
$\frac{\partial}{\partial \mathbf{u}_{i_n}^{(n)}}\big(x_{\alpha}-(\T{G}\times\{\mathbf{u}\}_{\alpha})\big)^2\\
=\frac{\partial}{\partial \mathbf{u}_{i_n}^{(n)}}tr\big(\big[x_{\alpha}-(\T{G}\times\{\mathbf{u}\}_{\alpha})\big]^{\mathsf{T}}\big[x_{\alpha}-(\T{G}\times\{\mathbf{u}\}_{\alpha})\big]\big)\\
=-2\frac{\partial}{\partial \mathbf{u}_{i_n}^{(n)}}tr\big(x_{\alpha}(\T{G}\times\{\mathbf{u}\}_{\alpha})\big)+\frac{\partial}{\partial\mathbf{u}_{i_n}^{(n)}}tr\big((\T{G}\times\{\mathbf{u}\}_{\alpha})^{\mathsf{T}}(\T{G}\times\{\mathbf{u}\}_{\alpha})\big)$
\begin{equation*}
\begin{split}
=&-2\frac{\partial}{\partial \mathbf{u}_{i_n}^{(n)}}tr\big(x_{\alpha}\mathbf{u}_{i_n}^{(n)}\mathbf{G}_{(n)}(\mathbf{u}_{i_N}^{(N)}\otimes\cdots\otimes\mathbf{u}_{i_{n+1}}^{(n+1)}\otimes\mathbf{u}_{i_{n-1}}^{(n-1)}\otimes\cdots\otimes\\
&\mathbf{u}_{i_{1}}^{(1)})^{\mathsf{T}}\big)+\frac{\partial}{\partial \mathbf{u}_{i_n}^{(n)}}tr\big(\big[\mathbf{u}_{i_n}^{(n)}\mathbf{G}_{(n)}(\mathbf{u}_{i_N}^{(N)}\otimes\cdots\otimes\mathbf{u}_{i_{n+1}}^{(n+1)}\otimes\mathbf{u}_{i_{n-1}}^{(n-1)}\otimes\cdots\\
&\otimes\mathbf{u}_{i_{1}}^{(1)})^{\mathsf{T}}\big]^{\mathsf{T}}\big[\mathbf{u}_{i_n}^{(n)}\mathbf{G}_{(n)}(\mathbf{u}_{i_N}^{(N)}\otimes\cdots\otimes\mathbf{u}_{i_{n+1}}^{(n+1)}\otimes\mathbf{u}_{i_{n-1}}^{(n-1)}\otimes\cdots\otimes\mathbf{u}_{i_{1}}^{(1)})^{\mathsf{T}}\big]\big)\\
=&-2x_{\alpha}\big[\mathbf{G}_{(n)}(\mathbf{u}_{i_N}^{(N)}\otimes\cdots\otimes\mathbf{u}_{i_{n+1}}^{(n+1)}\otimes\mathbf{u}_{i_{n-1}}^{(n-1)}\otimes\cdots\otimes\mathbf{u}_{i_{1}}^{(1)})^{\mathsf{T}}\big]^{\mathsf{T}}\\
&+2\mathbf{u}_{i_n}^{(n)}\mathbf{G}_{(n)}(\mathbf{u}_{i_N}^{(N)}\otimes\cdots\otimes\mathbf{u}_{i_{n+1}}^{(n+1)}\otimes\mathbf{u}_{i_{n-1}}^{(n-1)}\otimes\cdots\otimes\mathbf{u}_{i_{1}}^{(1)})^{\mathsf{T}}\big[\mathbf{G}_{(n)}\\
&(\mathbf{u}_{i_N}^{(N)}\otimes\cdots\otimes\mathbf{u}_{i_{n+1}}^{(n+1)}\otimes\mathbf{u}_{i_{n-1}}^{(n-1)}\otimes\cdots\otimes\mathbf{u}_{i_{1}}^{(1)})^{\mathsf{T}}\big]^{\mathsf{T}}\\
=&-2\big(x_{\alpha}-(\T{G}\times\{\mathbf{u}\}_{\alpha})\big)\big[(\T{G}\times_{-n}\{\mathbf{u}\}_{\alpha})_{(n)}\big]^{\mathsf{T}}
\end{split}
\end{equation*}
Other gradients of Equations \eqref{eqn:gradient} are calculated in similar manners.
